# Supplementary material for: Flexible Content Placement in Cache Networks using Reinforced Counters
Source: arXiv:1501.03446 source file (2015-03-18)
Supplement: Supplementary file 1 [file appendix-np.tex]

\section{Appendix B}

\begin{theorem} \label{theo1}
If different files have different sizes, the optimal content placement problem is NP hard.
\end{theorem}

\begin{proof}
Let us consider the problem of deciding if a  given content placement is optimal.   We refer to such decision problem as {\sc  Cache}.  Note that the problem of finding the optimal placement, i.e. the {\sc PlacementProblem}, must be harder than {\sc  Cache}, since solving the optimization problem yields  a solution to {\sc  Cache}.

We proceed with a reduction from the {\sc Knapsack} problem to {\sc Cache}.   An instance of the {\sc Knapsack}
 problem consists of
\begin{enumerate}
\item the capacity $c$ of the bag;
\item a set of $N$ elements, each with weight $w_i$ and value $v_i$, $1 \leq i \leq N$.
\end{enumerate}
The {\sc Knapsack} problem consists of deciding if a given set of items $\mathcal{I}$ maximizes the value carried in the bag under 
the constraint of their
net weight being smaller than the bag capacity $c$, $\sum_{i \in \mathcal{I}} w_i \leq c$.    This problem is known to be NP complete~\cite{introalg}.

An instance of {\sc Knapsack} can be mapped into an instance of {\sc Cache} comprised of 
two caches
 where cache 1 has capacity $c$ and serves file requests with exogenous arrival rates of $\lambda_{1j} = w_j$ whose sizes 
are $t_j$, $1 \leq j \leq N$ (see Figure~\ref{fig:np1}).

Given an instance $x=(c, N, (w_i), (v_i), \mathcal{I})$ of the {\sc Knapsack} problem we transform it into an 
instance $f(x)=(C, F, (s_i), (t_i), (\lambda_{ij}), (\mu_i), (A_{ij}), (M_{ij}))$ of the 
{\sc Cache} problem as follows.  Let $C=2$ and $F=N$. Let $t_i = w_i$, $i=1, \ldots, F$, $\lambda_{ij} = v_i$, $i=1, \ldots, F, j=1, 2$, and $\mu_i=\infty$, $i=1,\ldots, C$. The capacities
of the caches are $s_1=c$ and $s_2=\infty$. $M_{12}=1$ (and $M_{ij}=0$ for $(i,j)\neq (1,2)$).  Finally,

\begin{equation}
A_{ij}=
\begin{cases} 1, & \text{if } i \in \mathcal{I} \text{ or } j=2, \\
0, &\text{otherwise}
\end{cases}
\end{equation}

\begin{figure}[h!]
\center
\includegraphics[scale=0.4]{np1}
\caption{Content placement when files have different sizes is NP hard.}
\label{fig:np1}
\end{figure}

$(\Rightarrow)$ If $x \in$ {\sc Knapsack} then the elements in $\mathcal{I}$ maximize $\sum_{i \in I} v_i$  under the constraint $\sum_{i\in I} w_i \leq c$.  Correspondingly,  since  $\lambda_{i1} = v_i$, $t_i = w_i$, $A_{i1} = 1 \Leftrightarrow (i \in \mathcal{I})$ and
$s_1 = c$ then $\sum_{i \text{ s.t. } A_{i1}=1} \lambda_{i1}$ is maximized under the constraint $\sum_{i \text{ s.t. } A_{i1}=1} t_i \leq s_1$.  Therefore, $A$ characterizes the set of files that minimizes the sum of endogenous request rates across caches, and $f(x) \in $ {\sc Cache}.  

$(\Leftarrow)$  If $x  \notin$ {\sc Knapsack} then this is either because 1) the constraint $\sum_{i\in I} w_i \leq c$ is not satisfied or 2) there is another set of files $\mathcal{I'}$ such that $\sum_{i \in I'} v_i > \sum_{i \in I} v_i$.  In both cases, $f(x) \notin$ {\sc Cache}, since 1) the constraint $\sum_{i \text{ s.t. } A_{i1}=1} t_i \leq s_1$ will not be satisfied (see Definition~\ref{defini}-2) and 
2) $\sum_{i \text{ s.t. } A_{i1}=1} \lambda_{i1}$   will not be maximized, which means that the endogenous rates will not be minimized (see Definition~\ref{defini}-3).  \end{proof}

\begin{theorem}
If all files have the same size, the optimal content placement problem is NP hard.
\end{theorem}
\begin{proof}
We refer to {\sc FeasibleCache} as the problem of deciding if a given cache network admits a feasible content placement.
Note that the problem of finding the optimal placement, i.e. the {\sc PlacementProblem}, must be harder than {\sc  FeasibleCache}, 
since solving the optimization problem yields  a solution to {\sc  FeasibleCache}. 

An instance $y=(C,F,(s_i),(t_i),(\lambda_{ij}),(\mu_i), (M_{ij}))$ of the {\sc FeasibleCache} problem consists of $C$ caches and $F$
files, with sizes $(s_i)$ and $(t_i)$, respectively.  File $j$ is requested with rate $\lambda_{ij}$ at cache $i$, and cache $i$
has service capacity $\mu_i$ requests/s.  There is a link from cache $i$ to cache $j$ if and only if $M_{ij}=1$.

Consider a set $N$ of elements. Let $v_i$ be the value of the $i$-th element in the set, $1 \leq i \leq |N|$.  
Let the size of a set be the sum of the values of the elements in that set.   The {\sc Partition} problem consists of deciding if  there is a partition of  $N$ elements into two sets $\mathcal{I}$ and $N \setminus \mathcal{I}$  with equal sizes, i.e., $\sum_{i \in \mathcal{I}} v_i = \sum_{i \in N \setminus \mathcal{I}} v_i$.  This problem is known to be NP complete~\cite{garey}.    

We proceed with a Turing reduction from the {\sc Partition} problem to the {\sc FeasibleCache} problem.  

An instance $x=(N, (v_i))$ of the {\sc Partition} problem consists of
\begin{enumerate}
\item a set $N$ of elements;
\item a value $v_i$ associated to each element $i$, $1 \leq i \leq N$
\end{enumerate}

Let $\Lambda=\sum_{i=1}^N v_i$. An instance $x=(N, (v_i))$  of {\sc Partition} is mapped into $N+1$ instances of {\sc FeasibleCache}, 
$f_0(x), f_1(x), f_2(x), \ldots, f_N(x)$.  Each instance of {\sc FeasibleCache} 
is 
comprised of two caches whose storage capacities (sizes)  sum to $N$ and whose service capacities are $\mu_i = \Lambda/2$, $i=1,2$ (see Figure~\ref{fig:np2}).

\begin{figure}[h!]
\center
\includegraphics[scale=0.4]{np2}
\caption{Content placement when files have same size is NP hard.}
\label{fig:np2}
\end{figure}

The $m$-th instance of {\sc FeasibleCache}, $0 \leq m \leq N$, is $f_m(x)=(2,N,(s_1=m, s_2=N-m),(t_i=1),(\lambda_{ij}=v_i),(\mu_i=\Lambda/2), (M_{12}=M_{21}=1, M_{ij}=0 \text{ otherwise}))$.

Next, we will show that 
$x \in ${ \sc Partition} $\Leftrightarrow \exists m \text{ s. t. } f_m(x) \in ${ \sc FeasibleCache} (see Figure~\ref{figpart}).

\begin{figure}
\center
\includegraphics[scale=0.6]{partition}
\caption{Reduction from Partition to FeasibleCache.} \label{figpart}
\end{figure}

$(\Rightarrow)$ If $x \in $ {\sc Partition}  then the elements in $N$ can be partitioned into two sets 
$\mathcal{I}$ and $N \setminus \mathcal{I}$  such that  $\sum_{i \in \mathcal{I}} v_i = \sum_{i \in N \setminus \mathcal{I}} v_i$.  
Therefore, the files in $F$ can be partitioned into two sets such that 
$\sum_{i \in \mathcal{I}} \lambda_{i1}  = \sum_{i \in N \setminus \mathcal{I}} \lambda_{i2} = \Lambda/2$, 
the cache network is stable (see Definition~\ref{defini}-1) and $\exists m \text{ s. t. } f_m(x) \in $ {\sc FeasibleCache}.

$(\Leftarrow)$  If $x \notin $ {\sc Partition}  then the elements in $N$ cannot be partitioned into 
two sets with the same size.  Therefore, the files in $F$ cannot be partitioned into two sets such that 
$\sum_{i \in \mathcal{I}} \lambda_{i1}  = \sum_{i \in N \setminus \mathcal{I}} \lambda_{i2} = \Lambda/2$, 
the cache network does not admit a stable solution, hence $\forall m, f_m(x) \notin $ {\sc FeasibleCache}.

\end{proof}
