# Supplementary material for: Flexible Content Placement in Cache Networks using Reinforced Counters
Source: arXiv:1501.03446 source file (2015-03-18)
Supplement: Supplementary file 2 [file appendix.tex]

\section{Appendix A}

\begin{lemma}
The function $\phi(K)=\pi_{up}^{-1/(K+1)}$ is convex. \label{convex1}
\end{lemma}
\begin{proof}
The second derivative of $\phi(K)$ is given by
\begin{equation}
\frac{d^2 \phi(K)}{d^2 K}= -  \frac{\log(\pi_{up}) \left(2 (K+1) - \log(\pi_{up})\right)}{(K+1)^4 (\pi_{up})^{1/(K+1)}}
\end{equation} 
Therefore, $\frac{d^2 \phi(K)}{d^2 K}  > 0$ and $\phi(K)$ is convex.
\end{proof}

\begin{lemma}
The function $\omega(K)= \frac{1 }{ (\pi_{up})^{-1/(K+1)}-1} $ is convex. \label{convex2}
\end{lemma}
\begin{proof}
The sign of the second derivate of $\omega(K)$ is 
the sign of 
\begin{equation}
\pi_{up}^{1/(K+1)}(2K-\log(\pi_{up})+2)-(2K+\log(\pi_{up})+2)
\end{equation}
For $\omega(K)$ to be convex we must have
\begin{equation}
\delta(K)= \pi_{up}^{1/(K+1)}(2K-\log(\pi_{up})+2) - (2K+\log(\pi_{up})+2) \ge 0 \label{ineqdif}
\end{equation}
Note that  $\pi_{up}^{1/(K+1)}$ is an increasing function of $K$.

First, let us  verify that
the inequality above hold for $K=0$, i.e.,
\begin{equation}
\pi_{up}(-\log(\pi_{up})+2) \ge(\log(\pi_{up})+2)
\end{equation}
Indeed, the inequality above holds for $\pi_{up}=1$ and the 
difference $\pi_{up}(-\log(\pi_{up})+2) -(\log(\pi_{up})+2)$ is non-increasing  as  
a function of $\pi_{up}$ as far as $\log(\pi_{up}) \ge 1-1/\pi_{up}$, which is always the case for $0 \leq \pi_{up} \leq 1$.

Now, note that the second derivative of  $\delta(K)$ is non-negative,
given by
\begin{equation}
\frac{d^2 \delta(K)}{dK} = -\frac{\pi_{up}^{1/(K+1)} (\log(\pi_{up}))^3 }{(K+1)^4} \ge 0
\end{equation}
Therefore, $\delta(K)$ is convex, $\delta(0)  \ge 0$ and $\delta(\infty)=0$. 
Hence, \eqref{ineqdif} holds and the result follows. 
\end{proof}
